# Supplementary material for: Topological index for periodically driven time-reversal invariant 2D systems
Source: arXiv:1407.7747 ancillary file (2015-03-23)
Supplement: Supplementary file 1 [file index_paper_supplemental.pdf]

# Supplementary Materials: A topological index for periodically driven time-reversal invariant 2D systems

David Carpentier, Pierre Delplace,* Michel Fruchart, and Krzysztof Gawędzki
*Laboratoire de Physique, École Normale Supérieure de Lyon, 47 allée d'Italie, 69007 Lyon, France*
(Dated: March 23, 2015)

## ROBUSTNESS OF THE EDGE STATES TO SPIN-FLIP HOPPINGS

This section aims at showing more concretely how the spin-flip hopping terms are introduced in the model. On a specific example, we show how the quasi-energy spectrum evolves from a case with only half of the model (spin $\uparrow$ only, see Ref. [1]) to the case discussed in this Letter with two time-reversal copies coupled together by a time-reversal symmetric hopping term. We next show how the edge states are gaped when the time-reversal constraint of the evolution operator is not satisfied anymore. By extending the model, we finally illustrate the expected property that the $K$ index counts the parity of edge states (per edge) and not their number.

The model we consider is a split-time evolution on a square lattice. Such an evolution is described by a unitary operator $U(t,k)$, where $k$ denote the quasi-momentum. At each time this operator can be simply expressed as a finite product of evolution operators describing the previous steps $\alpha$, during which the Bloch Hamiltonian of the system $H_\alpha(k)$ is constant in time.

During each step $\alpha = 1 \ldots 5$ of the evolution, the Bloch Hamiltonian takes the general form

$$H_\alpha(k) = \begin{pmatrix} H_\alpha^{\uparrow\uparrow}(k) & H_\alpha^{\downarrow\uparrow}(k) \\ H_\alpha^{\uparrow\downarrow}(k) & H_\alpha^{\downarrow\downarrow}(k) \end{pmatrix} . \tag{S.1}$$

The TRI constraint $\Theta U(t,k)\Theta^{-1} = U(-t,-k)$ then implies $H^{\downarrow\downarrow}(t,k) = \overline{H}^{\uparrow\uparrow}(-t,-k)$ (the two spin copies are time-reversed symmetric to each other) and $H^{\uparrow\downarrow}(t,k) = -\overline{H}^{\downarrow\uparrow}(-t,-k)$. This second relation gives the rule to allow spin-flipping processes while keeping TRI and hence a well-defined $K$ index. Since we consider a split-step evolution, the off-diagonal spin-flipping parts of the Bloch Hamiltonian are related to each others as

$$\begin{aligned} H_5^{\uparrow\downarrow}(k) &= -\overline{H}_1^{\downarrow\uparrow}(-k) \\ H_4^{\uparrow\downarrow}(k) &= -\overline{H}_2^{\downarrow\uparrow}(-k) \\ H_3^{\uparrow\downarrow}(k) &= -\overline{H}_3^{\downarrow\uparrow}(-k) \ . \end{aligned} \tag{S.2}$$

In addition, hermiticity of $H_\alpha(k)$ must be satisfied at each time which imposes

$$H_\alpha^{\uparrow\downarrow}(k) = \overline{H}_\alpha^{\downarrow\uparrow}(k) \ . \tag{S.3}$$

One can now infer the explicit form of the matrices $H_\alpha^{\uparrow\downarrow}(k)$. In the infinite strip geometry, the dimension of these matrices corresponds to the number of sites $N$ across the width of the strip times the number $M$ of sites in the unit cell $m$ (called $A_m$ and $B_m$ in our case where $M = 2$). These $MN \times MN$ matrices thus read

$$H_1^{\uparrow\downarrow}(k_x) = J' \begin{array}{c} \begin{array}{cc} \uparrow A_m & \uparrow B_m \end{array} \\ \begin{pmatrix} \ddots & & & \\ & 0 & 1 & \\ & 1 & 0 & \\ & & & \ddots \end{pmatrix} \end{array} \begin{array}{l} \\ \downarrow A_m \\ \downarrow B_m \\ \end{array} \tag{S.4}$$

$$H_2^{\uparrow\downarrow}(k_x) = J' \begin{array}{c} \begin{array}{cccc} \uparrow A_{m-1} & \uparrow B_{m-1} & \uparrow A_m & \uparrow B_m \end{array} \\ \begin{pmatrix} \ddots & & & & & \\ & 0 & 0 & 0 & -\mathrm{e}^{\mathrm{i}k_x} & \\ & 0 & 0 & 0 & 0 & \\ & 0 & 0 & 0 & 0 & \\ & \mathrm{e}^{\mathrm{i}k_x} & 0 & 0 & 0 & \\ & & & & & \ddots \end{pmatrix} \end{array} \begin{array}{r} \\ \downarrow A_{m-1} \\ \downarrow B_{m-1} \\ \downarrow A_m \\ \downarrow B_m \\ \end{array} \tag{S.5}$$

$$H_3^{\uparrow\downarrow}(k_x) = J' \begin{array}{c} \begin{array}{cc} \uparrow A_m & \uparrow B_m \end{array} \\ \begin{pmatrix} \ddots & & & \\ & 0 & -\mathrm{e}^{2\mathrm{i}k_x} & \\ & \mathrm{e}^{2\mathrm{i}k_x} & 0 & \\ & & & \ddots \end{pmatrix} \end{array} \begin{array}{l} \\ \downarrow A_m \\ \downarrow B_m \\ \end{array} \tag{S.6}$$

$H_4^{\uparrow\downarrow}(k_x)$ and $H_5^{\uparrow\downarrow}(k_x)$ being given by the TRI constraint. The Floquet operator whose spectrum gives the quasi-energies is finally given by

$$U(T,k_x) = U_5(k_x)U_4(k_x)U_3(k_x)U_2(k_x)U_1(k_x) \tag{S.7}$$

where $U_\alpha$ is the evolution operator at the end of the step $\alpha$.

In Figure 1, we show how the quasi-energy spectrum is modified when the coupling between spins is introduced. Figure 1 (a) shows the quasi-energy spectrum for the spin $\uparrow$ periodic dynamics only, for the strip geometry with a specified choice of parameters (see Ref. [1]). The $W$ index defined in the $\pi$ gap can be computed and is found to be $W_\pi = 1$ in agreement with the existence of one chiral state at each edge of the strip. Indeed, the

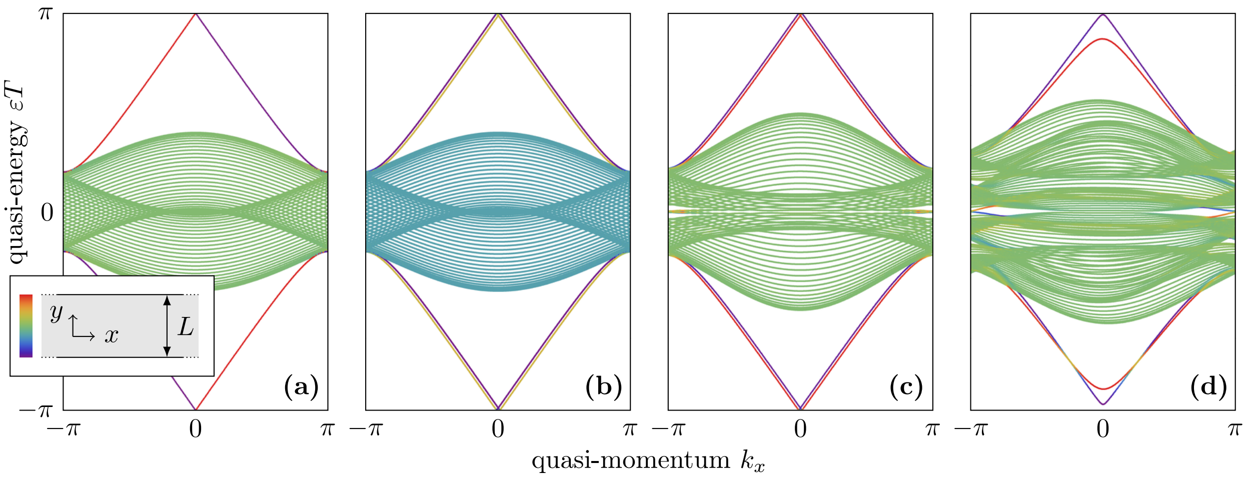


FIG. 1. Quasi-energy spectra for a strip geometry (inset) for $J = 3\pi$ and $\Delta = 0$. We consider (a) spin ↑ only (see Ref. [1]), (b) spin ↑ and spin ↓ with no coupling ($J' = 0$), (c) spin ↑ and spin ↓ with $J' = 1/2$, (d) spin ↑ and spin ↓ with $J' = 1/2$ and time-reversal breaking term.

bulk gap of quasi-energy hosts one chiral edge state at each edge of the ribbon. Next, we add the TR copy (spin ↓) to the previous case. the spectrum we obtain in Fig. 1 (b) simply consists in the superposisition of the sepctrum of Fig. 1 (a) and its TR copy (given by $k \to -k$). The bulk quasi-energy gap thus simply hosts two uncoupled counter-propagating chiral edge states (a small boundary mass term is added to distinguish them), and the value of the $K$ index is given by the simplified formula (8) of main text, that yields $K_\pi = 1$. In Fig. 1 (c), the TRI spin-flipping term of amplitude $J'$ has been introduced. This reproduces the Fig. 3 (a) of the main text. The width of the quasienergy gap has reduced but remained positive. This coupling did not effect the presence of a pair of edge states whose existence is in agreement with the $K$ index which could not change value. Finally, in Fig. 1 (d), we have introduced a spin-flip term that breaks TRI during one step of the evolution. More precisely, we have imposed $H_5^{\uparrow\downarrow}(k) = +\overline{H}_1^{\downarrow\uparrow}(-k)$. As expected, the crossing point of the edge states at $k = 0$ is not protected anymore by the Kramers theorem and the degeneracy is lifted.

Next, we illustrate the fact that the $K$ index counts the parity of the number of pairs of edge states similarly to the KM index in the static case.

For that purpose, we consider a TRI evolution with two time-reversed copies of periodic evolutions characterized by $W_\pi = 3$. To generate such an evolution, we extend the initial model by introducing hopping terms $J_2$ between further nearest neigbours, as depicted in 2(a). Such a model allows more than one pair of edge states (per edge). The introduction of a perturbation that maintains time-reversal symmetry, such as the spin-flip hopping term $J'$ (which now couples the same sites that $J_2$ does), may eventually gap out the crossings of the edge states which do not occur at a time-reversal symmetry point. Typically, the system will therefore not necessarily support the same number of edge states in a given quasi-energy gap, as illustrated in Fig. 2(b). However, the parity of this number cannot change and is in agreement with the value of the $K$ index, $K_\pi = 1$.

## EXISTENCE OF THE CONTRACTION

In general, the obstructions to the existence of a contraction of a map $V$ from BZ to $U(2M)$ to the constant map equal to Id are non-trivial winding numbers of $\det V$. Here, we want to contract the map $V = V_\epsilon(T/2, \cdot)$ to the identity with a time-reversal constraint :

$$\Theta V(t,k)\Theta^{-1} = V(t,-k) \qquad \text{(S.8)}$$

To do so, consider first the restriction of this map to a half of the Brillouin zone $\text{BZ}^+$ such that $k_x \in [0,\pi]$. This half Brillouin zone can be seen as a cylinder, whose boundary is composed of two circles $\mathcal{C}_0$ and $\mathcal{C}_\pi$ which are stable under $k \to -k$. Hence, we can further restrict the map $V$ to each of the circles $\mathcal{C}$ (independently). Now, $\mathcal{C}$ itself is composed of two halves related by $k \to -k$, so we can consider only one half $\mathcal{C}^+$, which we contract to the identity. In order to preserve the time-reversal constraint Eq. S.8, this contraction has to be done carefully: at the end-points $P_0, P_\pi = \partial\mathcal{C}^+$ of the half-circle, $V$ is a symplectic matrix. As the symplectic group is simply connected, there is a path connecting $V(P_0)$ (resp. $V(P_\pi)$) to the identity, so we can complete the path in $U(2M)$ to a loop which can then be contracted to the group identity (after some calculations, the only obstruction to do so happens to be the windings of $\det V$ around

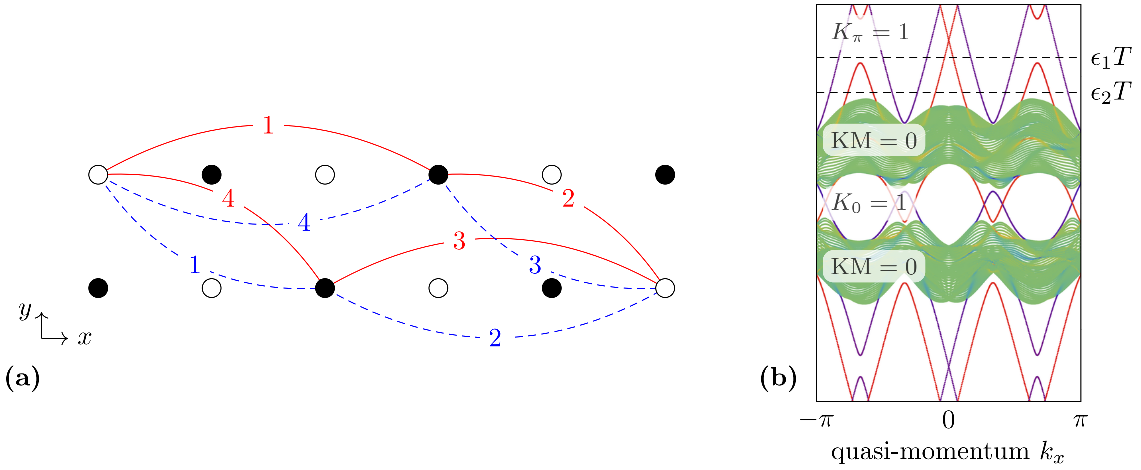


FIG. 2. (a) Extended lattice model with hopping terms $J_2$, spin up (red solid lines) and spin down (blue dashed lines). For clarity, the hoppings are not all drawn. (b) Quasi-energy spectrum of the extended lattice model for a ribbon geometry with $J_2 = 5\pi/2$, $J = 0$, $\Delta = \pi$ and $J' = 1$. The number of edge states in a gap is not the same at quasi-energies $\epsilon_1$ and $\epsilon_2$, but the parity is well given by the $K$ index.

the Brillouin zone, which are trivial). Then, copying this contraction to the other half of $\mathcal{C}$, one obtains a time-reversal preserving contraction on the whole boundary of the cylinder. Gluing these contractions to the initial map produces a map from the 2-sphere to unitary operators, with poles mapped to the identity. Without the additional constraint that poles remain mapped to the identity, such a map is contractible, and in our specific case, the constraint does not obstruct the contraction. Hence, we can deform the corresponding map to the constant map equal to the identity, and, using time-reversal, a contraction of the map from the whole Brillouin zone to the unitary group is obtained.

## THE $\boldsymbol{Z}_2$ NATURE OF THE $K$ INDEX

We have explained that it is indeed possible to find contractions of Eq. (S.8) of the family of operators $V(T/2, k)$. Writing down an explicit contraction is not always straightforward, and a systematic procedure is still lacking. Moreover, such a contraction is not unique. A natural question is whether the index $K$ depends on the choice of the contraction or not. In other terms, is this index really well-defined? The reason that as a $\boldsymbol{Z}_2$-valued quantity $K$ does not depend of the choice of contraction is that for two different choices the integrals defining K would differ by an even number. In the following we sketch a proof of the above assertion which explains why such integrals do not define an integer-valued index.

Let us call $K$ and $K'$ the values of the integral in (7) calculated with two different contractions. The difference $K - K'$ can be written as the degree of a periodic map $V$ starting and ending at Id and satisfying the constraint Eq. S.8 at all times. We have to show that the degree of such a map is always an even integer. First, time-reversal ensures that the integral over BZ is twice the integral on $\text{BZ}^+$. Thus, it remains to show that the integral on $\text{BZ}^+$ is an integer. This is not obvious because the manifold $\mathcal{M} = S^1 \times \text{BZ}_+$ on which the integral is carried out has boundaries ($S^1 \sim [0, T]$ describing one period of time, i.e. it is $[0, T]$ with boundaries identified). To circumvent this difficulty, we extend the restriction $V_{|\mathcal{M}}$ of $V$ to $\mathcal{M}$ to a map $\tilde{V}$ defined on a closed manifold, such that the extension does not contribute to the integral. To do so, we consider the boundary of $\mathcal{M}$ which is composed of two tori $\mathcal{T}_0$ and $\mathcal{T}_\pi$. Let us then work on one of these tori, say $\mathcal{T}_0$. At first sight, $V$ is identically equal to the identity at $t = 0$, so we can pinch the meridian $t = 0$ of $\mathcal{T}_0$ to a point and $V_{|\mathcal{M}}$ is effectively a map from the sphere. As $\pi_2(U(2M))$ is trivial, this map can indeed be contracted to the identity. However, it is not obvious whether it can be contracted to the identity while respecting the time-reversal invariant constraint (S.8). Let us show that it is indeed possible: first, consider the torus $\mathcal{T}_0$ as a rectangle with opposite boundaries identified, parametrized by $t$ and $k_y$. The boundaries at $t = 0$ and $t = T$ are identically mapped to the identity. Now, the images of the boundaries at $k_y = 0$ and $k_y = \pi$ of the half of the rectangle corresponding to $k_y \geq 0$ are inside the symplectic group, which is simply connected. Henceforth, the restriction of $V$ to the whole boundary of the half-rectangle is mapped to $Sp(2M)$ and can therefore be contracted to the identity inside the symplectic group (this means that the time-reversal invariant constraint (S.8) is satisfied). We end up with a map from a 2-sphere to the unitary group with poles mapped to the identity, and this map can indeed be contracted to the constant map equal to the identity. This contraction, that we call

$\widetilde{V}_0$, satisfies the time-reversal invariant constraint (S.8) (provided the poles stay mapped e.g. to the identity all along). We obtain this way a contraction of $V$ restricted to the half torus $\mathcal{T}_0$ which may be extended to the one, denoted $\widetilde{V}_0$, of $V$ restricted to $\mathcal{T}_0$ by the time-reversal constraint (S8). Similarly, for the torus $\mathcal{T}_\pi$, we obtain a contraction $\widetilde{V}_\pi$. We may glue $\widetilde{V}_0$, $V|_\mathcal{M}$ et $\widetilde{V}_\pi$ to get a map from a closed surface (pictorially, $\mathcal{M}$ with properly capped boundaries). Finally, time-reversal invariance on the boudnaries of $\mathcal{M}$, which, by construction, extends to the caps, ensures that the contributions to the degree from $\widetilde{V}_0$ and $\widetilde{V}_\pi$ vanish, hence the conclusion.

For more details, see [2].

* Corresponding author : pierre.delplace@ens-lyon.fr

[1] M. S. Rudner, N. H. Lindner, E. Berg, and M. Levin, Phys. Rev. X **3**, 031005 (2013), 1212.3324.

[2] D. Carpentier, P. Delplace, M. Fruchart, K. Gawędzki, and C. Tauber, ArXiv e-prints (2015), 1503.04157.
